# Supplementary material for: Positional Encoding Augmented GAN for the Assessment of Wind Flow for Pedestrian Comfort in Urban Areas
Source: arXiv:2112.08447 source file (2022-01-04)
Supplement: Supplementary file 1 [file 01-additional-abstract.tex]

% Graphical abstract
\begin{graphicalabstract}
\includegraphics[width=1.0\textwidth]{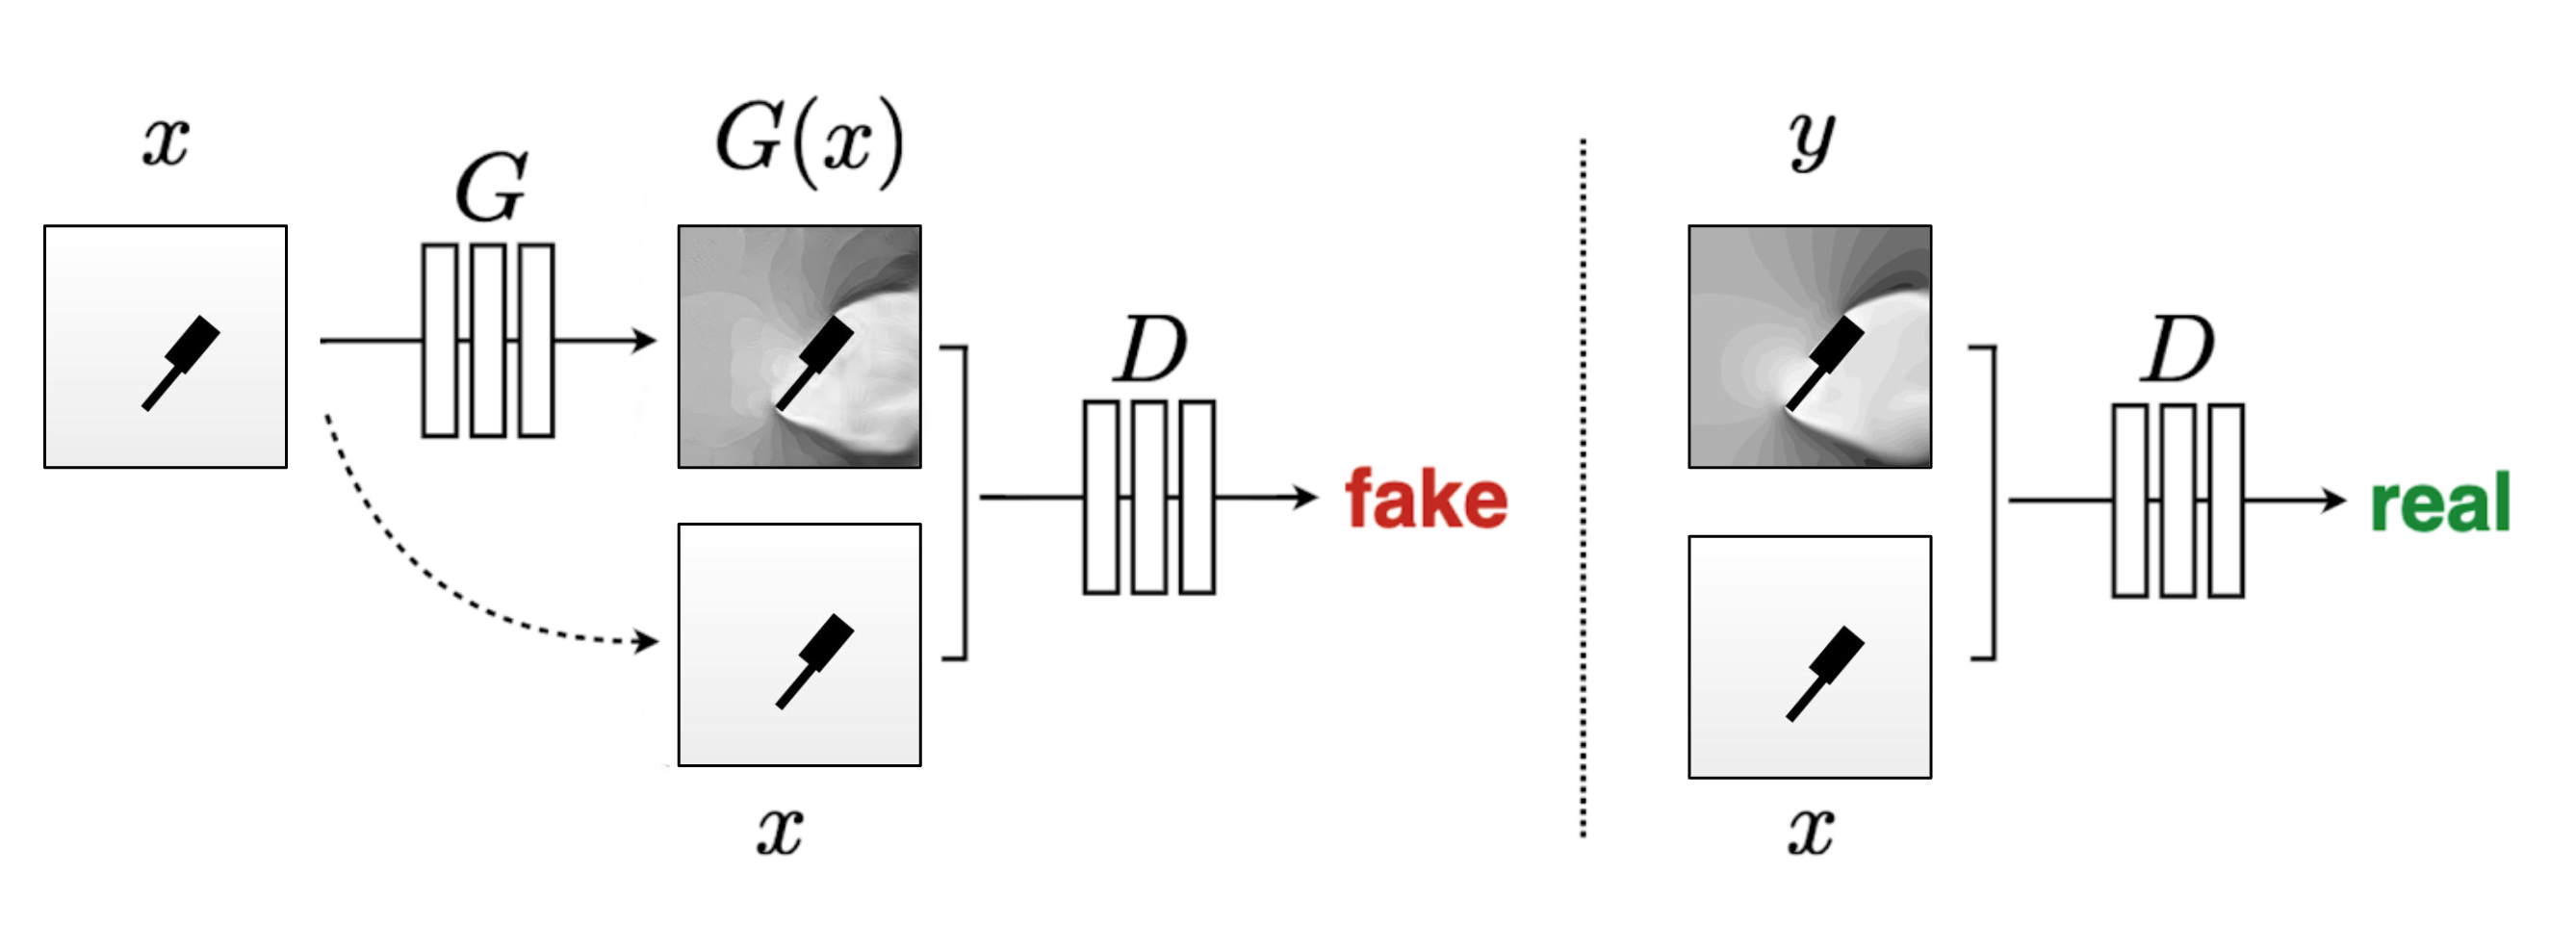}
\end{graphicalabstract}

% Hightlights
\begin{highlights}
\item Using state-of-the art GAN architectures for image-to-image translation to learn the underlying RANS equations from fluid dynamics.
\item Injecting positional information into the architectures improves results
\item ...??
\end{highlights}
